# Supplementary material for: Mixed Degradation Image Restoration via Local Dynamic Optimization and Conditional Embedding
Source: arXiv:2411.16217 source file (2024-11-25)
Supplement: Supplementary file 1 [file X_suppl.tex]

\clearpage
\setcounter{page}{1}
\maketitlesupplementary
\section{Comparison of Inference Speed}
To evaluate the image processing speed of various methods, we tested each method on 100 images of size 256$\times$256 and calculated the average processing speed per image. The detailed results are shown in Table~\ref{tab:speed}. It can be observed that Transformer-based methods are generally slower in inference compared to CNN-based methods. Additionally, our method demonstrates an advantage in processing performance.

\begin{table}[h]
\centering
\setlength{\tabcolsep}{1pt}
\caption{Comparison of the number of parameters, FLOPs, and Speed.}
\begin{tabular}{ccccccc} 
\hline
Methods  & AirNet & PromptIR & Restormer & IRNext & AST   & Ours  \\ 
\hline
Para.(M) & 9.0    & 33.0     & 24.5      & 13.2   & 110.3 & 8.9   \\
FLOPs(G) & 77.9   & 158.1    & 174.7     & 114.0  & 65.3  & 71.5  \\
Speed(s) & 0.039   & 0.088    & 0.083     & 0.025  & 0.065  & 0.026  \\
\hline
\end{tabular}
\label{tab:speed}
\end{table}

\section{Dataset Generation Process}

The Flickr2K dataset is employed as the source of pristine, degradation-free images. After a meticulous selection process, we selected 1,359 pristine images representing diverse and richly detailed scenes. To simulate degraded scenarios, images were generated for four single degradation types and three mixed degradation types based on the selected clean images. Each degradation category consists of 1,359 pairs of degraded and clean images, with 1,200 pairs allocated for training and 159 pairs reserved for testing. The degraded images were generated via programmatic implementation, ensuring the diversity and realism of the degraded image distribution.

\subsection{Single Degradation Type Generation}

\subsubsection{\textbf{Noise Degradation}}
Noise degradation is achieved by combining random noise and illumination effects, and is computed as follows:
\begin{equation}
I_{\text{noise}} = \text{clip}\left(\frac{I}{L} \cdot L^{\alpha} + \mathcal{N}(0, \sigma), 0, 1\right),
\end{equation}
where \(I\) denotes the input image, \(L\) represents the illumination map (refined and smoothed using guided filtering), and \(\alpha\) is a parameter controlling illumination intensity, randomly sampled from \([2, 3]\). \(\mathcal{N}(0, \sigma)\) denotes Gaussian noise with zero mean and a standard deviation \(\sigma\), where \(\sigma \in [0.03, 0.08]\).

\subsubsection{\textbf{Haze Degradation}}
Haze degradation is simulated based on the atmospheric scattering model, expressed as:
\begin{equation}
I_{\text{haze}} = I \cdot t + A \cdot (1 - t),
\end{equation}
where
\begin{equation}
t = e^{-\beta \cdot d}.
\end{equation}
Here, \(d\) represents the depth map (obtained using MegaDepth~\cite{MDLi18}), which models scene depth variation, and \(\beta \in [1.0, 2.0]\) denotes the atmospheric attenuation coefficient. \(A\) is the global atmospheric light intensity, randomly sampled from \([0.6, 0.9]\). By adjusting the transmittance \(t\) and atmospheric light \(A\), haze effects of varying densities and color distributions are simulated.

\subsubsection{\textbf{Rain Degradation}}
Rain degradation is simulated by superimposing a rain mask~\cite{Garg:2006:PRR:1179352.1141985} onto the image:
\begin{equation}
I_{\text{rain}} = \text{clip}(I + M_{\text{rain}}, 0, 1),
\end{equation}
where \(M_{\text{rain}}\) is a rain mask randomly selected from a rain mask library. The mask is binarized and resized to match the resolution of the input image, resulting in visually consistent rain streak textures.

\subsubsection{\textbf{Snow Degradation}}
Snow degradation is simulated by overlaying a snow mask~\cite{liu2018desnownet} onto the image:
\begin{equation}
I_{\text{snow}} = I \cdot (1 - M_{\text{snow}}) + C \cdot M_{\text{snow}},
\end{equation}
where \(M_{\text{snow}}\) is a snow mask with randomly controlled distribution, and \(C\) represents the snow intensity, empirically set to \(1.01\). This formulation blends the snow and background regions to approximate realistic snow-covered scenes.

\subsection{Mixed Degradation Type Generation}
Mixed degradation scenarios are simulated by sequentially applying the transformations corresponding to the single degradation types.

\textbf{Rain\_Haze:} Simulated by successively applying the rain mask and the haze atmospheric scattering model.

\textbf{Haze\_Noise:} Simulated by successively applying the haze atmospheric scattering model and Gaussian noise.

\textbf{Rain\_Haze\_Noise:} Simulated by successively applying the rain mask, haze atmospheric scattering model, and Gaussian noise.
